# Supplementary material for: What's in your hands? 3D Reconstruction of Generic Objects in Hands
Source: arXiv:2204.07153 source file (2022-04-14)
Supplement: Supplementary file 1 [file todo_appendix.tex]

\section*{Appendix}
\paragraph{Objectives.}
In the end, we hope to have one among:
\begin{itemize}
    \item A system that uses single image, with hand+object segmentation, to predict: a) Hand pose (including articulation), b) Object 3D

    \item A system that can use a video clip of interaction with noisy hand-object segmentation, to predict: a) Hand pose (including articulation), b) Object 3D, c) Possibly improved segmentation
\end{itemize}

To achieve either goals, we need:
\begin{itemize}
    \item Articulation-conditioned Shape Prior
    \item Differentiable rendering + contact objectives
    \item Diverse video or image data showing hand-object interactions, with not-too-bad segmentation.
    \item Open question: will the inference approach be optimization-only? Or can we learn from real videos and images? It would be pretty cool if we can!
\end{itemize}

\newpage
\paragraph{Timeline.}
A slightly optimistic timeline:

\vspace{2mm} \noindent \emph{Mid-to-end August:}
\begin{itemize}
    \item Finalize the articulation-conditioned shape model (at least the architecture + training methodology, if not the final data etc.)
    \item Prepare a presentation of what we have so far in context of the objectives above (in terms of data, approach, results)
    \item Identify baselines
\end{itemize}

\vspace{1mm} \noindent \emph{Early-to-Mid Sept:}
\begin{itemize}
    \item Initial image/video based optimization results on limited categories
    \item Initial contact optimization results
    \item Identify diverse data sources (is 100DOH + CoCo segmentation enough?). Hopefully 10k or so independent interaction clips (or images)?
\end{itemize}

\vspace{1mm} \noindent \emph{Mid-to-End Sept:}
\begin{itemize}
    \item Ablate and finalize optimization strategy
    \item Mine and process all image/video data we might need.
    \item Initial results for some baselines on limited data
\end{itemize}

\vspace{1mm} \noindent \emph{Early-to-Mid Oct:}
\begin{itemize}
    \item Results for baselines
    \item Optimization results on all data (outputs: shape and articulation)
    \item At this stage, our results should be publishable on their own i.e. reconstruction of generic objects
\end{itemize}

\vspace{1mm} \noindent \emph{Mid-to-End Oct:}
\begin{itemize}
    \item Make amazing visualizations
    \item Initial paper writing + figures
    \item Can approach improve with learning from unlabelled data?
    \item Can the optimized results be pseudo-GT for single view prediction?
\end{itemize}

\vspace{1mm} \noindent \emph{Early-to-Mid Nov:}
\begin{itemize}
    \item Finalize any learning experiments
    \item Make amazing webpages
    \item Finish paper
\end{itemize}
